# Supplementary material for: An Analysis by Synthesis Method that Allows Accurate Spatial Modeling of Thickness of Cortical Bone from Clinical QCT
Source: arXiv:2009.08664 ancillary file (2020-09-18)
Supplement: Supplementary file 1 [file supplement.pdf]

# An Analysis by Synthesis Method that Allows Accurate Spatial Modeling of Thickness of Cortical Bone from Clinical QCT

Stefan Reinhold[1]✉, Timo Damm[3], Sebastian Büsse[2], Stanislav N. Gorb[2], Claus-C. Glüer[3], and Reinhard Koch[1]

[1] Department of Computer Science, Kiel University, Kiel, Germany
{sre,rk}@informatik.uni-kiel.de
[2] Functional Morphology and Biomechanics, Institute of Zoology, Kiel University, Kiel, Germany
{sbuesse,sgorb}@zoologie.uni-kiel.de
[3] Section Biomedical Imaging, Molecular Imaging North Competence Center (MOIN CC), Department of Radiology and Neuroradiology, University Medical Center Schleswig-Holstein (UKSH), Kiel University, Kiel, Germany
{timo.damm,glueer}@rad.uni-kiel.de

## 6 Supplement

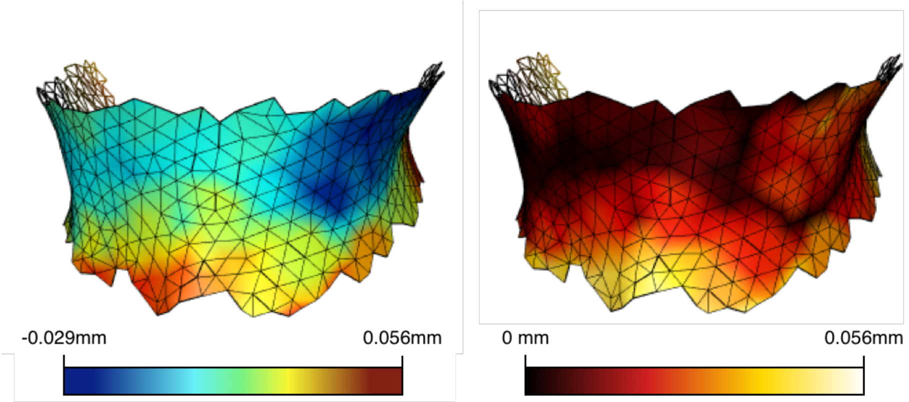


Fig. 4: Visualization of the spatial distribution of the differences (left: signed, right: absolute) between estimated AbS based Ct.Th and HR-pQCT wCt.Th gold standard for a representative vertebra.

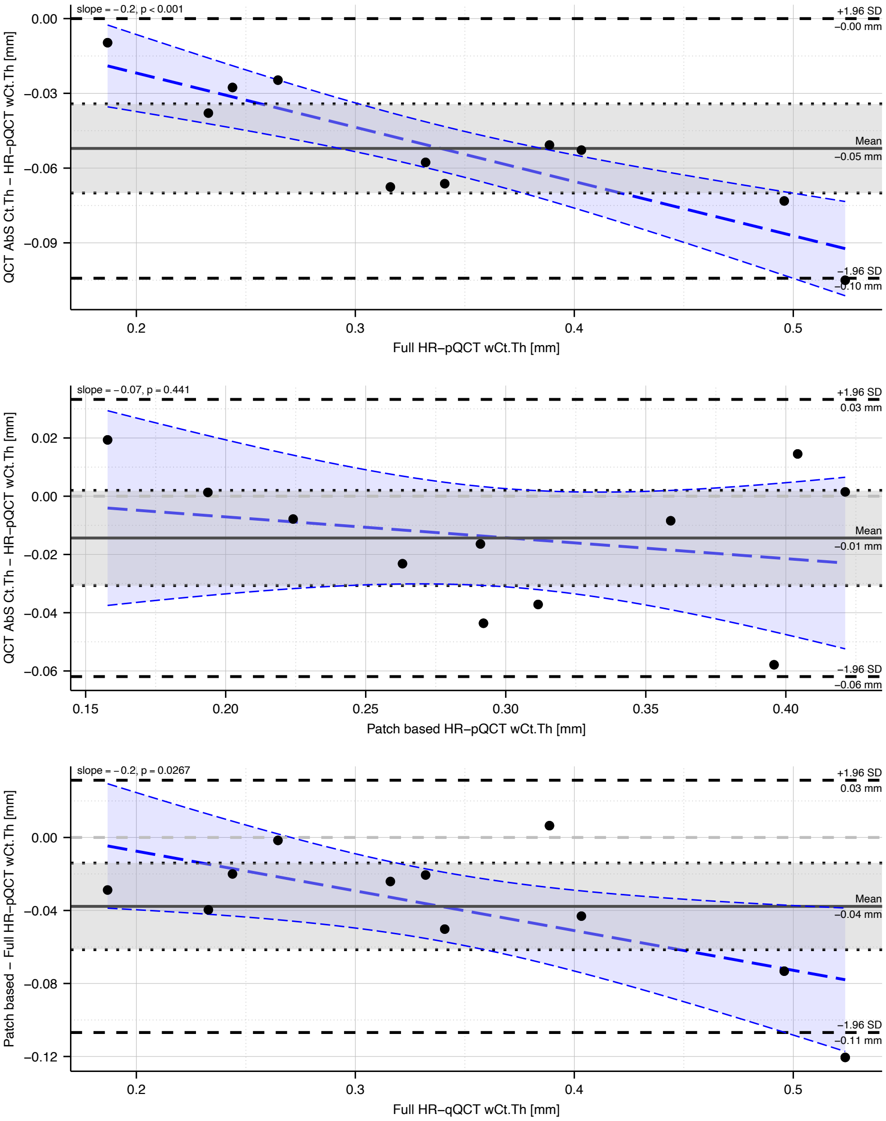


Fig. 5: Modified Bland-Altman plots. Top: AbS method vs. full HR-pQCT wCt.Th gold standard. The significant slope indicates a proportional error, however AbS was evaluated on only 48 patches, full HR-pQCT wCt.Th on the complete vertical cortex. Center: AbS method vs. patch based HR-pQCT wCt.Th; the proportional error vanishes. Bottom: patch based HR-pQCT wCt.Th vs. full HR-pQCT wCt.Th. The same slope as in the top row is visible, supporting our hypothesis, that the proportional error is induced by the different samples.

Table 3: CT protocol settings.

| | | QCT | HR-pQCT | HR-µCT |
|---|---|---|---|---|
| Device | | Somatom 64 | XtremeCT | Skyscan1172 |
| Manufacturer | | Siemens | Scanco | Bruker |
| In-plane pixel size | [µm] | 234 | 82 | 1.73 |
| Slice width | [µm] | 1000 | 82 | 1.73 |
| Voltage | [kV] | 120 | 60 | 59 |
| Exposure | [mA s] | 100 | 190 | 720 |
| Kernel | | B40s | Standard | Standard |

Table 4: Prior parameters used for the proposed AbS method. For each $(\mu, \sigma)^{\mathrm{T}} \sim \mathrm{NI}\chi^2 : \ \mu \sim \mathcal{N}(\mu_0, \sigma^2\kappa^{-1})$ and $\sigma^2 \sim$ Scale-inv-$\chi^2(\nu, \sigma_0^2)$

| Region | Metric | | $\mu_0$ | $\kappa$ | $\nu$ | $\sigma_0$ |
|---|---|---|---|---|---|---|
| Cortex | Log Thickness | [log mm] | -1.6 | 0.01 | 0.01 | 0.5 |
| Cortex | Density | [mg cm$^{-3}$] | 1200.0 | 0.01 | 0.10 | 50.0 |
| Spongiosa | Density | [mg cm$^{-3}$] | 150.0 | 10.00 | 10.00 | 150.0 |
| Background | Density | [mg cm$^{-3}$] | 10.0 | 50.00 | 1.00 | 10.0 |
| Cortex | Distance | [mm] | 0.0 | 0.01 | 0.10 | 0.5 |

Table 5: Start parameters for our AbS algorithm. Other parameters were: $\sigma_\epsilon = 100, \sigma_\xi = 10, K = 50000$.

| Region | Metric | | $\mu$ | $\sigma$ |
|---|---|---|---|---|
| Background | Density | [mg cm$^{-3}$] | 10.00 | 10.00 |
| Cortex | Density | [mg cm$^{-3}$] | 1200.00 | 200.00 |
| Spongiosa | Density | [mg cm$^{-3}$] | 150.00 | 20.00 |
| Cortex | Log Thickness | [log mm] | -1.61 | 0.50 |
| Cortex | Distance | [mm] | 0.00 | 0.10 |
